# Supplementary material for: A Tale of Two Scales: Reconciling Horizontal and Vertical Scaling for Inference Serving Systems
Source: arXiv:2407.14843 source file (2024-07-20)
Supplement: Supplementary file 1 [file appendix.tex]

\section{Appendix}
\label{sec:appendix}
